# Supplementary material for: Self-organization and cyclic positioning of active condensates
Source: arXiv:2510.15771 source file (2026-06-05)
Supplement: Supplementary file 1 [file SM.pdf]

# Supplemental Material for
# Self-Organization and Cyclic Positioning of Active Condensates

Hossein Vahid,[1] Jens-Uwe Sommer,[1,2,*] and Abhinav Sharma[3,1,†]

[1] *Leibniz-Institut für Polymerforschung Dresden, Bereich Theorie der Polymere, 01069 Dresden, Germany*
[2] *Technische Universität Dresden, Institut für Theoretische Physik, 01069 Dresden, Germany*
[3] *Faculty of Mathematics, Natural Sciences, and Materials Engineering: Institute of Physics, University of Augsburg, Universitätsstraße 1, 86159 Augsburg, Germany*

## SI. LIQUID-VAPOR COEXISTENCE

To generate vapor-liquid coexistence configurations of active Brownian particles (ABPs), we employ a direct coexistence protocol adapted from prior studies of phase-separating systems [1–3]. Initially, 2500 ABPs are equilibrated in a periodic cubic box of dimensions $80 \times 80 \times 80$. The system is then uniformly compressed to a smaller cube $(15 \times 15 \times 15)$ to have a homogeneous condensed phase. After equilibration, the box is instantaneously expanded along the $z$-axis to span the interval $z \in [-40, 40]$, while keeping the transverse box dimensions fixed. This procedure generates a dense slab near the midplane $(-7.5 \lesssim z \lesssim 7.5)$ surrounded by low-density regions (vapor regions). 10 additional ABPs are randomly placed in the vapor region. For each value of the attraction strength $\epsilon$, the system is equilibrated for $2 \times 10^6$ time steps, followed by an additional $2 \times 10^7$ steps for data sampling.

The steady-state time-averaged density profile $\rho(z)$ is calculated along the $z$-axis, normal to the vapor–liquid slab. Figure S1(a) presents $\rho(z)$ at Pe = 10 for varying $\epsilon$. The systems exhibit distinct liquid and vapor regions, with the vapor density decreasing as $\epsilon$ increases. To extract the coexisting liquid and vapor densities $\rho_\ell$ and $\rho_v$, as well as the interface positions and interfacial width $d$, the density profiles were fitted to a two-interface *double-tanh* function,

$$\rho(z) = \rho_v + \frac{\rho_\ell - \rho_v}{2}\left[\tanh\left(\frac{z - z_1}{d}\right) - \tanh\left(\frac{z - z_2}{d}\right)\right], \tag{S1}$$

where $z_1$ and $z_2$ indicate the two vapor–liquid interfaces. Nonlinear least-squares fitting using the Levenberg–Marquardt algorithm is employed to extract the best-estimate parameters $\{\rho_\ell, \rho_v, z_1, z_2, d\}$, with typical fitting uncertainties in $\rho_\ell$ and $\rho_v$ below $10^{-4}$. The coexistence densities are fitted by modeling the average and the difference between the liquid and vapor branches. Specifically, the average density $\bar{\rho} = \frac{1}{2}(\rho_\ell + \rho_v)$ and density difference $\Delta\rho = (\rho_\ell - \rho_v)$ are fitted as

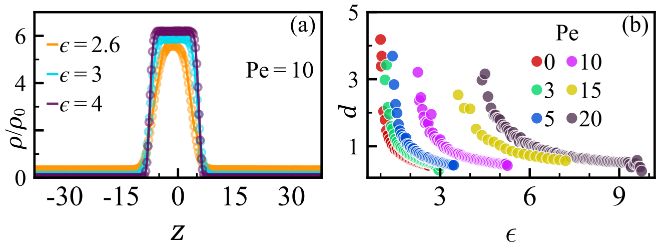


FIG. S1. (a) Steady-state density profiles $\rho(z)$ at varying $\epsilon$ for Pe = 10, showing coexistence between dense and dilute regions. (b) Interfacial width $d$ as a function of $\epsilon$ for various Pe values, indicating sharper interfaces at stronger attractions.

$$\bar{\rho} = \rho^* + A\left(\frac{1}{\epsilon^*} - \frac{1}{\epsilon}\right) \quad \text{and} \quad \Delta\rho = \Delta\rho_0\left(1 - \frac{\epsilon^*}{\epsilon}\right)^\lambda \tag{S2}$$

where $\rho^*$ is the critical density, $\epsilon^*$ is the critical attraction strength, and $A$ and $\Delta\rho_0$ are fitting parameters. The exponent $\lambda$ is varied between 0.2 and 0.3 to achieve the best fit to the simulation data.

Fig. 1 of the main manuscript shows the phase diagrams as functions of the attraction strength $\epsilon$ for varying Pe. The interfacial width $d$, shown in Fig. S1(b), decreases systematically with increasing $\epsilon$ for all Pe values. This trend is consistent with the expectation that stronger attractions sharpen the interface between the liquid and vapor phases by suppressing interfacial fluctuations. At lower $\epsilon$, the interfaces are broader due to enhanced particle mobility and interfacial roughness, while at higher $\epsilon$, the condensed phase becomes more tightly bound, leading to narrower interfaces.

Table SI summarizes the fitted critical densities $\rho^*$ and attraction strengths $\epsilon^*$ as a function of Pe. Both $\rho^*$ and $\epsilon^*$ increase with activity, indicating that higher densities and stronger attractions are required to stabilize a liquid phase at larger Pe. For Pe = 0, the extracted values ($\rho^* \approx 0.31$, $\epsilon^* \approx 0.96$) are consistent with results for similar short-range attractive systems [2, 4].

## SII. CONDENSATE COARSENING

To investigate the coarsening dynamics of ABPs, we perform simulations for 5000 attractive ABPs randomly

* jens-uwe.sommer@tu-dresden.de
† abhinav.sharma@uni-a.de

TABLE SI. Estimated critical density $\rho^*$ and critical attraction strength $\epsilon^*$ at different Pe.

| Pe | 0 | 3 | 5 | 10 | 15 | 20 |
|---|---|---|---|---|---|---|
| $\rho^*$ | 0.31 | 0.33 | 0.36 | 0.40 | 0.41 | 0.42 |
| $\epsilon^*$ | 0.96 | 1.13 | 1.37 | 2.17 | 3.27 | 4.14 |

distributed in a periodic cubic box of size $50^3$. For each Pe, three independent simulations are performed, and each run lasts for $2\times10^8$ time steps. Particle positions are recorded every 2000 steps. Clusters are identified based on a distance criterion: particles within a cutoff of 1.4, corresponding to the first minimum of the radial distribution function after the primary peak, are considered connected. At each recorded frame, the size-weighted mean cluster size was calculated as $\langle N_c\rangle = \sum_i (N_\mathrm{c}^i)^2/\sum_i N_\mathrm{c}^i$, where $N_\mathrm{c}^i$ denotes the number of particles of the $i$-th cluster.

Figure S2 shows the time evolution of $\langle N_\mathrm{c}\rangle$ for attractive ABPs. In panel (a), the attraction strength is fixed at $\epsilon = 3$, while Pe is varied from 0 to 8. Increasing Pe leads to faster growth of $\langle N_c\rangle$, indicating that activity enhances droplet mobility and promotes coalescence. While this trend could partly originate from the lower liquid densities at higher Pe, as denser clusters typically exhibit slower dynamics [5], the results in panel (b) indicate otherwise. At fixed $\epsilon/\epsilon^* = 2$, the coarsening remains faster for larger Pe despite the liquid phase being equally or even more dense (see Fig. S1(b)). This supports the conclusion that activity plays a dominant role in enhancing coarsening by increasing cluster mobility.

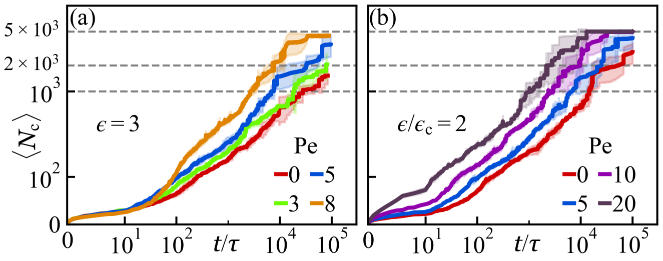


FIG. S2. Time evolution of $\langle N_\mathrm{c}\rangle$ for 5000 attractive ABPs at different Péclet numbers Pe with (a) fixed attraction strength $\epsilon = 3$, and (b) $\epsilon/\epsilon^* = 2$ (see Table SI for $\epsilon^*$ values). Shaded areas indicate standard deviation across three independent simulations. Increasing Pe accelerates coarsening, indicating that active droplets are more mobile and coalesce more rapidly.

## SIII. ABPS IN ACTIVITY GRADIENT

We perform simulations for 5000 ABPs in an activity field given by $f_\mathrm{a}(z) = f_\mathrm{a}^*(z+25)/50$ (same protocols as in Fig. 3 of the main manuscript). ABPs are initially placed at random within a $50\times50\times50$ box. Periodic boundary conditions are imposed in the $x$ and $y$ directions, while ABP are confined between two purely repulsive harmonic walls positioned at $z = -25$ and $z = 25$. The planar walls interact with ABPs via a purely repulsive harmonic potential, $E = 4(d - r_\mathrm{c})^2$. This repulsion acts only when the particle's shortest distance to the wall $d$ is less than the interaction range $r_\mathrm{c} = 2\sigma$. Each simulation lasts $3\times10^8$ time steps, and the final $10^8$ steps are used for data analysis.

Figure S3 shows the normalized density profiles $\rho(z)/\rho_0$ of ABPs along the activity gradient for increasing $f_\mathrm{a}^*$ values and various attraction strengths $\epsilon$. Across all gradients, we observe that particle accumulation is highly sensitive to both the propulsion strength and interparticle cohesion. At the weakest gradient ($f_\mathrm{a}^* = 10$, Fig. S3(a)), condensates are stable for $\epsilon \geq 3$ and localize in high activity regions ($z > +10$). For lower cohesion ($\epsilon = 1, 2$), the system fails to condense, and particles remain in a dispersed gas-like state, accumulating preferentially in the low-activity region ($z < 0$).

As the activity gradient steepens ($f_\mathrm{a}^* = 20$ and 40; Figs. S3(b,c)), the tendency for low-$\epsilon$ systems to disperse is enhanced due to increased particle evaporation from weakly bound clusters. For moderate $\epsilon$, we observe the formation of living clusters that nucleate in the low-activity region and migrate toward higher activity. However, the cohesive strength is insufficient to maintain cluster integrity at high propulsion, leading to cluster fragmentation and broad density distributions. The steady-state density peaks are at intermediate activity regions. In the strongest gradient case ($f_\mathrm{a}^* = 80$, Fig. S3(d)), only the most cohesive systems ($\epsilon \geq 4$) show significant clustering. These clusters remain highly localized near the low-activity end, suggesting that the intense propulsion at higher $z$ rapidly disrupts any condensate that attempts to migrate to higher activity regions. Consequently, the system enters a regime where only strong cohesion can sustain partial clustering, while weaker attractions are overwhelmed by activity-induced dispersion.

To further characterize the dynamical stability of clusters formed by attractive ABPs under spatial activity gradients, we analyze cluster size (number of ABPs closer than 1.4) transition matrices $P(N_1 \mid N_0, \Delta t)$, which represent the conditional probability that a cluster of initial size $N_0$ evolves to a size $N_1$ after a fixed time interval $\Delta t = 20\tau$. Figure S4 displays these matrices for a range of attraction strengths $\epsilon \in \{1, 2, 3, 4\}$ and activity gradient magnitudes $f_\mathrm{a}^* \in \{10, 20, 40, 80\}$. For weak cohesion ($\epsilon = 1$; left column), clusters are generally unstable across all gradient strengths. However, as the activity gradient steepens (from top to bottom), we observe enhanced accumulation of ABPs in low-activity regions (see Fig. S3), which facilitates the formation of transient larger clusters in low-activity regions. This is depicted in a gradual upward extension of the distribution along the $N_0$ and $N_1$ axes, particularly for $f_\mathrm{a}^* = 40$ and 80. Despite their size, these clusters remain fragile and short-lived, as indicated by the spread away from the diagonal, consistent with high rates of evaporation and recondensation.

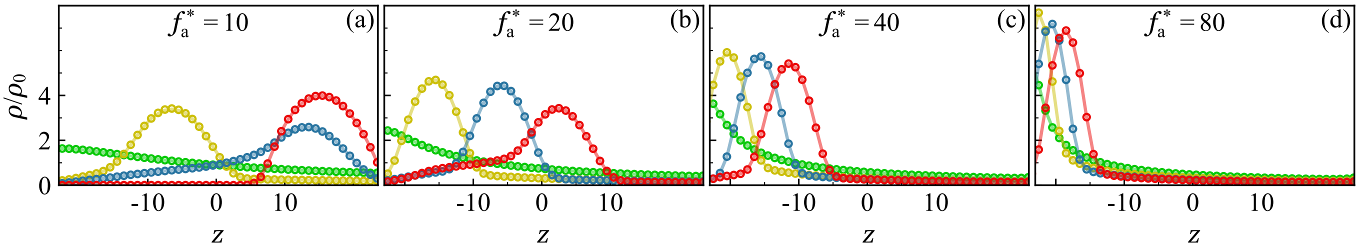

FIG. S3. ((a)-(d) steady state density profile of ABPs along the z axis for varying $\epsilon$. The activity field is given by $f_a(z) = f_a^*(z+25)/50$, and the system along the z-axis is non-periodic. The density is normalized by the mean initial density $\rho_0$.

At moderate attraction ($\epsilon = 2$ and 3; middle columns), a diagonal structure emerges in the transition matrices, indicating that clusters tend to retain their size over short time intervals. However, the distributions remain somewhat diffuse, reflecting frequent cluster merging and fragmentation. As $f_a^*$ increases, the distribution becomes broader and more asymmetric, consistent with activity-driven instabilities that promote size fluctuations. For strong attraction ($\epsilon = 4$; rightmost column), the matrices are sharply peaked along the diagonal, especially for lower $f_a^*$, indicating highly stable condensates with minimal fluctuations. In the extreme case of $f_a^* = 10$ and $\epsilon = 4$ (Fig. S4(d)), the cluster retains nearly all ABPs. As $f_a^*$ increases, even strong clusters become more dynamic due to enhanced propulsion, broadening the matrix and allowing transitions between cluster sizes.

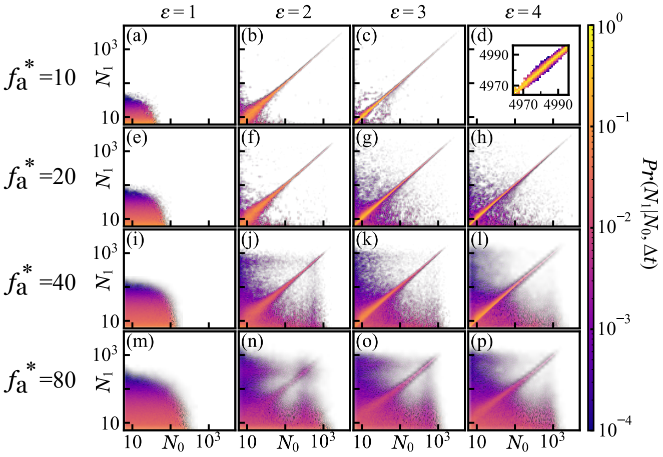

FIG. S4. Transition matrices $P(N_1 \mid N_0, \Delta t)$ showing the conditional probability that a cluster of initial size $N_0$ evolves to size $N_1$ after a time interval $\Delta t = 20\tau$, for various attraction strengths $\epsilon$ and activity gradient magnitudes $f_a^*$. Panels correspond to: (a)–(d) $f_a^* = 10$, (e)–(h) $f_a^* = 20$, (i)–(l) $f_a^* = 40$, and (m)–(p) $f_a^* = 80$, with increasing $\epsilon$ from left to right ($\epsilon = 1$ to 4). Color intensity denotes the probability on a logarithmic scale (see color bar). The diagonal structure reflects cluster size persistence, while the spread away from the diagonal indicates dynamical fluctuations due to aggregation and fragmentation.

## SIV. COMPUTATIONAL DETAILS FOR PASSIVE DROPLETS IN A TEMPERATURE GRADIENT AND ACTIVE DROPLETS IN AN ACTIVITY GRADIENT

A condensate of $N = 950$ attractive particles ($\epsilon = 2$) is simulated in a periodic box of dimensions $L_x = L_y = 10.4\,\sigma$ and $L_z = 30\,\sigma$. The droplet is prepared in equilibrium and then placed at $z = 15$, i.e. at the interface between two regions of different temperatures. To create a stationary thermal gradient, every $10^4$ integration steps we add non-translational kinetic energy at a constant rate $\dot{Q} = 10^{-3}\,\varepsilon/\tau$ to all particles in the *hot* slab at $15 < z < 30$, and remove the same amount from the *cold* slab $0 < z < 15$. Because the energy is distributed uniformly within each slab, total linear momentum is conserved. The equations of motion are integrated in the $NVE$ ensemble with a velocity-Verlet scheme and a time step $5 \times 10^{-4}\,\tau$. The imposed heat flux establishes a linear temperature profile along the $z$–axis. The droplet drifts into the cooler half $0 < z < 15\,\sigma$ and remains there for the remainder of the simulation.

For ABPs, we perform simulations for two different types of clusters, each with $N = 950$ ABPs in a periodic box of dimensions $L_x = L_y = 10.4\,\sigma$ and $L_z = 30\,\sigma$. First, for the attractive condensates, ABPs interact using the Wang–Frenkel potential (as in the main manuscript) with $\epsilon = 2$. A pre-equilibrated droplet was placed at $z = 15$ , at the interface of a step-gradient in activity (Pe $= 0$ for $z \in \{0, 15\}$ and Pe $= 5$ for $z \in \{15, 30\}$). Second, for the the motility-induced phase separation (MIPS) simulations, ABPs interact via the purely repulsive Weeks–Chandler–Andersen (WCA) potential. The pre-equilibrated cluster is also placed at $z = 15$ but is exposed to a much stronger activity gradient (Pe $= 0$ for $z \in \{0, 15\}$ and Pe $= 120$ for $z \in \{15, 30\}$). The WCA potential is defined as:

$$U_{\mathrm{WCA}}(r) = 4\epsilon_{\mathrm{WCA}}\left[\left(\frac{\sigma}{r}\right)^{12} - \left(\frac{\sigma}{r}\right)^{6} + \frac{1}{4}\right]\Theta(r_c - r)\,, \tag{S3}$$

where $\epsilon_{\mathrm{WCA}} = 1$ is the potential well depth, $\sigma = 1$ the interaction diameter, $\Theta(\cdot)$ the Heaviside step function, and the cutoff is $r_c^{ij} = 2^{1/6}\sigma$.

## SV. MIXTURE OF ACTIVE BROWNIAN PARTICLES

Physical interactions are fundamental to morphogenesis in cell biology [6–8], as exemplified by the differential adhesion hypothesis. This principle describes how cells self-sort based on adhesion strength, with more cohesive cells forming a core that is enveloped by less cohesive ones [9–13]. The physical intelligence inherent in this mechanism has already inspired control algorithms for robot swarms [14–16]. Motivated by this, we investigate whether this sorting principle can be mapped onto ABP systems. To this end, we perform simulations of a binary mixture containing $N = 5000$ particles of two types, $\alpha$ and $\beta$, where $\chi$ represents the fraction of $\beta$ particles. Type-$\alpha$ particles are ABPs with a self-interaction strength of $\epsilon^{\alpha\alpha} = 4$. Type-$\beta$ particles are ABPs with a self-interaction strength of $\epsilon^{\beta\beta} = 2$ (Fig. S5). The cross-interaction strength between the two types is set to $\epsilon^{\alpha\beta} = 3$, with all interactions governed by the WF potential. The activity field is given by $f_{\mathrm{a}}(z) = 20(z + 25)/50$, and the system is non-periodic along the $z$-axis.

Figure S5(a) shows the steady-state particle density profiles along the $z$-axis for varying $\chi$. As $\chi$ increases, the peak of the total particle density shifts monotonically toward the lower activity region (i.e., lower $z$). This behavior interpolates between the two pure-component limits. The cases of $\chi = 0$ (only $\alpha$-particles) and $\chi = 1$ (only $\beta$-particles) reproduce the behavior shown previously in Fig. 3 of main manuscript. The simulation snapshots and corresponding pair correlation functions $g(r)$ (Figures S5(b-d)) provide a microscopic picture of the system self-organization, driven by differential cohesive interactions. Visually, the system undergoes micro-phase separation, where the strongly-attractive $\alpha$-particles (blue) form dense, condensed cores. These cores are surrounded by the weakly-attractive $\beta$-particles (orange). Notably, this surrounding layer is asymmetric, with more $\beta$-particles accumulating on the side of the clusters facing low-activity regions. The extremely sharp and high peaks in $g^{\alpha\alpha}$ signify a dense, highly-correlated structure resulting from strong self-attraction. The demixing of the two particle types is confirmed by the $g^{\alpha\beta}$ peak, which is significantly lower than the $g^{\alpha\alpha}$ peak, even at $\chi = 0.8$. Moreover, as $\chi$ increases, the $g^{\alpha\alpha}$ peak grows taller. It indicates that the $\alpha$-clusters are compressed into a more densely packed and ordered state, which we attribute to the increased effective pressure exerted by the surrounding fluid of $\beta$-particles.

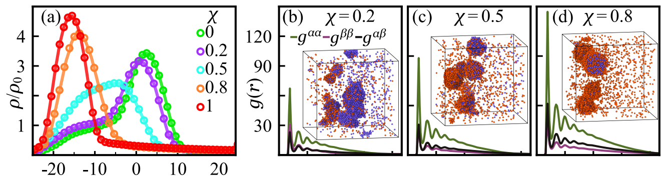


FIG. S5. Binary mixtures of ABPs. A fraction $1-\chi$ of ABPs are $\alpha$-type ($\epsilon^{\alpha\alpha} = 4$) and a fraction $\chi$ are $\beta$-type ($\epsilon^{\beta\beta} = 2$). (a) Steady–state density $\rho(z)$. (b–d) Pair correlations $g^{ij}(r)$ with corresponding snapshots.


[S1] M. C. Muniz, T. E. Gartner, M. Riera, C. Knight, S. Yue, F. Paesani, and A. Z. Panagiotopoulos, J. Chem. Phys. **154**, 10.1063/5.0050068 (2021).

[S2] V. Prymidis, S. Paliwal, M. Dijkstra, and L. Filion, J. Chem. Phys. **145**, 10.1063/1.4963191 (2016).

[S3] A. K. Omar, Z.-G. Wang, and J. F. Brady, Phys. Rev. E **101**, 012604 (2020).

[S4] X. Wang, S. Ramírez-Hinestrosa, J. Dobnikar, and D. Frenkel, Phys. Chem. Chem. Phys. **22**, 10624 (2020).

[S5] J. Varennes, B. Han, and A. Mugler, Biophys. J. **111**, 640 (2016).

[S6] C.-P. Heisenberg and Y. Bellaïche, Cell **153**, 948 (2013).

[S7] B. Ladoux and R.-M. Mège, Nat. Rev. Mol. Cell Biol. **18**, 743 (2017).

[S8] A. Dance, Nature **589**, 186 (2021).

[S9] R. A. Foty and M. S. Steinberg, Dev. Biol. **278**, 255 (2005).

[S10] L. Chanson, D. Brownfield, J. C. Garbe, I. Kuhn, M. R. Stampfer, M. J. Bissell, and M. A. LaBarge, Proc. Natl. Acad. Sci. **108**, 3264 (2011).

[S11] A. E. Cerchiari, J. C. Garbe, N. Y. Jee, M. E. Todhunter, K. E. Broaders, D. M. Peehl, T. A. Desai, M. A. LaBarge, M. Thomson, and Z. J. Gartner, Proc. Natl. Acad. Sci. **112**, 2287 (2015).

[S12] S. Toda, L. R. Blauch, S. K. Tang, L. Morsut, and W. A. Lim, Science **361**, 156 (2018).

[S13] S. Wang, K. Matsumoto, S. R. Lish, A. X. Cartagena-Rivera, and K. M. Yamada, Cell **184**, 3702 (2021).

[S14] V. G. Santos, A. G. Pires, R. J. Alitappeh, P. A. Rezeck, L. C. Pimenta, D. G. Macharet, and L. Chaimowicz, Swarm Intell. **14**, 259 (2020).

[S15] S. Ceron, G. Gardi, K. Petersen, and M. Sitti, Proc. Natl. Acad. Sci. **120**, e2221913120 (2023).

[S16] M. Pan, Y. Yang, X. Qin, G. Li, N. Xi, M. Long, L. Jiang, T. Zhao, and L. Liu, Cell Rep. Phys. Sci. **5**, 10.1016/j.xcrp.2024.102122 (2024).
